# Supplementary material for: Differentiation of Linear Optical Circuits
Source: arXiv:2401.07997 source file (2024-12-08)
Supplement: Supplementary file 1 [file appendix.tex]

\section{QPath diagrams}

The sequential and parallel composition of these matrices are given
as follows:
$$\scalebox{0.85}{\tikzfig{figures/composition}}$$
By selecting and copying the rows of $A$ accoding to $I$ and $J$ we may construct
a matrix $A_{I, J} : n_I + m \to n_J + m'$ where
$n_I = \sum_{x=1}^k I_x$ and $n_J = \sum_{y=1}^{k'} I_y$.
This is done by applying the following diagrammatic rules:
$$\tikzfig{figures/merge-split}$$
where $\scalebox{0.8}{\tikzfig{figures/qpath/generators/merge}}$ denotes the matrix $\begin{pmatrix} 1 \\ 1 \end{pmatrix}$
and $\scalebox{0.8}{\tikzfig{figures/qpath/generators/split}}$ denotes $\begin{pmatrix} 1 & 1 \end{pmatrix}$.
These rules introduce positive real numbers as scalars, called \emph{normalisation},
which multiply under parallel or sequential composition.
They can be applied until the diagram is reduced to a normal form with only single particle creations and annihilations:
$$\tikzfig{figures/normal-form}$$
where $N_{I, J} = \sqrt{\prod_{x} I_x! \prod_y I_y!}$.

\section{Dilation of the number operator}

$$A = \begin{pmatrix} 0 & 1 \\ 1 & 1 \end{pmatrix}$$
$$ s = \sqrt{\frac{3 + \sqrt{5}}{2}}$$
$$U = \begin{pmatrix} -\frac{A^\dagger}{s} & D \\ D & \frac{A}{s} \end{pmatrix}$$
$$D = \begin{pmatrix} \alpha s^2 & - \alpha s \\ - \alpha s & \alpha \end{pmatrix}$$
$$ \alpha = \frac{\sqrt{1 - \frac{1}{s^4}}}{s^2 + 1} $$
$$A_m = \begin{pmatrix} 0 & 0 & \dots & 0 & 1\\ 0 & 1 & & 0 & 0\\ \vdots & & \ddots & & \vdots\\ 0 & 0 & & 1 & 0\\ 1 & 0 & \dots & 0 & 1 \end{pmatrix}$$
$$D_m = \begin{pmatrix} \alpha s^2 & 0 & \dots & 0 & - \alpha s \\ 0 & \beta & & 0 & 0 \\ \vdots & & \ddots & & \vdots \\ 0 & 0 & & \beta & 0\\ - \alpha s & 0 & \dots & 0 & \alpha \end{pmatrix}$$
$$ \beta = \sqrt{1 - \frac{1}{s^2}} $$
$$U_m = \begin{pmatrix} -\frac{A_m^\dagger}{s} & D_n \\ D_n & \frac{A_m}{s} \end{pmatrix}$$
$$\scalebox{0.8}{\tikzfig{figures/example-fig}}$$

\section{Differentiation of an amplitude}

Consider the phase operator $e^{i \hat{n} \theta}$, the derivative is easily written as an operator:
$$ \frac{d}{d\theta} e^{i \hat{n} \theta} = i \hat{n} e^{i \hat{n} \theta}$$
We may also express this as the following diagrammatic equation:
$$\tikzfig{figures/diff-phase}$$
where we use a blue box to denote the differentiation operator and the $\frac{\pi}{2}$ phase shift is introduced 
to account for the factor of $i$.
Now, suppose we want to compute the derivative of a circuit $C(\theta): m \to m$ with a single occurence of a 
phase shift with parameter $\theta$. The following derivation shows that the derivative can be computed as a QPath 
diagram $(M(\theta), [1], [1]): m + 1 \to m + 1$ with one ancillary photon.
$$\scalebox{0.7}{\tikzfig{figures/diff-circuit}}$$
Note that, since $\hat{n}$ is not unitary, the matrix $M(\theta)$ cannot be unitary. In fact, $\hat{n}$ 
is an unbounded operator, so $M(\theta)$ is not even a contraction. However, using Theorem~\ref{thm-dilation}, 
we can construct a unitary $U(\theta) : 2(m + 1) \to 2(m + 1)$ such that for any $I, J \in \mathbb{N}^m$:
\begin{equation}
    \frac{d}{d\theta} \bra{J} C(\theta) \ket{I} = \bra{1, J} M(\theta) \ket{1, I} = \norm{M(\theta)}^N \bra{1, J, \vec{0}} U(\theta) \ket{1, I, \vec{0}}
\end{equation}
where $N = \mathtt{sum}(I)$ is the number of input photons and $\vec{0}$ is a list of zeros of size $m + 1$.
Therefore we can compute the derivative of the amplitudes of $C(\theta)$ by post-selecting from the unitary circuit $U(\theta)$ and rescaling the results.

In the case where multiple phase shifts with parameter $\theta$ appear in the circuit, the derivative is computed 
by using the product rule. This requires computing the amplitude of one linear optical circuit for each occurence 
of the parameter and then summing the results. Since QPath diagrams are not closed under addition, we believe it is unlickely that a single 
linear optical circuit can be used to compute the derivative when $\theta$ appears multiple times.
Note that our procedure only computes the derivative with respect to one parameter in the circuit. In order to 
obtain the gradient, we must repeat the procedure for each distinct parameter.

\section{Second term of the expectation}

$$\scalebox{0.7}{\tikzfig{figures/diff-expectation2}} $$

\section{Tket talk}

$H$

$$\mathcal{F}(H) = \bigoplus_{n=0}^\infty H^{\tilde{\otimes} n}$$

$$ \mathcal{F}(f \oplus g) = \mathcal{F}(f) \otimes \mathcal{F}(g) $$

$$ \eta: H \to  \mathcal{F}(H) $$

$$ - \frac{1}{2}\left(\frac{\abs{\braket{\psi}{\phi}}^2}{2} - \frac{1}{2}\right) 
+ \frac{1}{2} \left(\frac{1}{2} - \frac{\abs{\braket{\psi}{\phi}}^2}{2}\right) \,
= \, \frac{1}{2} - \frac{\abs{\braket{\psi}{\phi}}^2}{2} $$
$$\tikzfig{figures/qpath}$$
$$\tikzfig{figures/distinguishability}$$

$$\tikzfig{figures/protocols} $$
$$\tikzfig{figures/fusion-network} $$
